# Supplementary material for: LoCo: Low-Bit Communication Adaptor for Large-scale Model Training
Source: arXiv:2407.04480 source file (2024-11-29)
Supplement: Supplementary file 1 [file appendix.tex]

\section{Discussion on Convergence Results}\label{sec:diss}
\subsection{Discussion about Lower Bound}
For the lower bound, as proven in~\cite{arjevani2020second}, on the nonconvex problems with Lipschitz gradient and Hessian,  for   stochastic gradient-based methods with {1) unbiased and 
variance-bounded stochastic gradient and 2) stochastic gradient queried on the same point per iteration}, their  complexity  lower bound  is  $\Omega(\epsilon^{-3.5})$ to find  an $\epsilon$-accurate first-order stationary point.  For condition 2), it means that per iteration, the algorithm only queries  the stochastic gradient at one point (e.g. SGD, Adam, Adan) instead of multiple points (variance-reduced algorithms, e.g. SVRG~\cite{johnson2013accelerating}). Otherwise, the   complexity  lower bound  becomes  $\Omega(\epsilon^{-3.0})$~\cite{arjevani2020second}.

For the nonconvex problems with Lipschitz gradient \emph{but without} Lipschitz Hessian, the complexity lower bound  is $\Theta(\epsilon^{-4})$ as shown in~\cite{arjevani2019lower}.  
Note, the above  Lipschitz gradient and Hessian assumption are defined on the training loss w.r.t. the variable/parameter instead of w.r.t. each datum/input $\zeta$. 
We would like to clarify that our proofs are only based on the above Lipschitz gradient and Hessian  assumptions and do not require  the Lipschitz gradient and Hessian w.r.t. the datum/input $\zeta$. 

\subsection{Discussion about Convergence Complexity}
The constant-level difference among the complexities of compared optimizers is not incremental.
Firstly, under the corresponding assumptions,  most  compared optimizers already achieve the optimal  complexity in terms of the dependence on optimization accuracy  $\epsilon$, and their complexities only differ  from their  constant factors, \eg $c_2$, $c_\infty$ and $d$.  For instance,  with Lipschitz gradient but without Lipschitz Hessian,  most optimizers have complexity $\order{\frac{x}{\epsilon^{4}}}$ which matches the lower bound $\order{\frac{1}{\epsilon^{4}}}$ in~\cite{arjevani2019lower}, where the  constant factor $x$  varies from different optimizers, \eg $x=c_{\infty}^2 d $ in Adam-type optimizer, $x=c_2^6$ in Adabelief,   $x = c_2^2d$  in LAMB, and $x=c_{\infty}^{2.5}$ in Adan.  So under the same conditions, one cannot improve  the complexity dependence on $\epsilon$ but can improve the constant factors which, as discussed below, is still significant, especially for  DNNs. 
	
Secondly, the constant-level difference may cause very different complexity whose magnitudes vary by several orders on networks.  This is because 1) the modern network is often large, e.g. 11 M parameters in the small ReNet18, leading a very large $d$; 2) for network gradient, its $\ell_2$-norm upper bound  $c_2$ is often much larger than its $\ell_\infty$-norm upper bound $c_\infty$ as observed and  proved in some work~\cite{du2018algorithmic},  because the stochastic  algorithms can probably adaptively adjust the parameter magnitude at different layers so that these parameter magnitudes are balanced.  
	
Actually, we also empirically find $c_\infty = \order{8.2}, c_2 = \order{430}, d = 2.2\times 10^{7}$ in the  ViT-small  across different optimizers, e.g., AdamW, Adam, Adan, LAMB.  In the extreme case, under the widely used  Lipschitz gradient assumption,  the complexity bound of Adan is $7.6\times 10^{6}$ smaller than the one of Adam, $3.3\times 10^{13}$ smaller than the one of AdaBlief, $2.1\times 10^{10}$ smaller than the one of LAMB, \etc.  For ResNet50, we also observe $c_\infty = \order{78}, c_2 = \order{970}, d = 2.5\times 10^{7}$ which also means a large big improvement of Adan over other optimizers.

\section{Additional Experimental Results}\label{sec:add-exp}

\subsection{Implementation Details of Adan}
%\noindent{\textbf{Implementation Details of Adan.}} 
For fairness, in all experiments, we only replace the optimizer with Adan and tune the  step size, warm-up epochs, and weight decay while fixing the other hyper-parameters, \eg~data augmentation, $\epsilon$ for adaptive optimizers, and  model parameters. Moreover, to make Adan simple, in all experiments except Table~\ref{tab:restart} in Sec.~\ref{restart}, we do not use the restart strategy.  
For the large-batch training experiment, we use the sqrt rule  to scale the learning rate:  $\text{lr} \!=\! \sqrt{\frac{\text{batch size}}{256} }\times 6.25$e-3, and respectively set warmup epochs $\{20,40,60,100,160,200\}$ for batch size $\text{bs}=\{1k,2k,4k,8k,16k,32k\}$.
For other remaining experiments, we use the hyper-parameters:  learning rate $1.5$e-2 for ViT/Swin/ResNet/ConvNext and MAE fine-tuning,  and $2.0$e-3 for MAE pre-training according to the official settings. 
We set $\beta_1 = 0.02, \beta_2 = 0.08$ and $\beta_3 = 0.01$, and let weight decay be $0.02$ unless noted otherwise. 
We clip the global gradient norm to $5$ for ResNet and do not clip the gradient for ViT, Swin, ConvNext, and {MAE}.
In the implementation, to keep consistent with Adam-type optimizers, we utilize the de-bias strategy for Adan.

\subsection{Detailed Comparison on ViTs}\label{sec:vit-more}
Besides AdamW, we also compare Adan with several other popular optimizers, including Adam, SGD-M, and LAMB, on ViT-S.  Table \ref{tab:vit-s} shows that SGD, Adam, and LAMB perform poorly on ViT-S, which is also observed in the  works~\cite{xiao2021early, nado2021large}. 
These results demonstrate that  the decoupled weight decay in Adan and AdamW is much more effective  than 1) the vanilla weight decay, namely the commonly used $\ell_2$ regularization in SGD, and 2) the one without any  weight decay, since as shown in Eqn.~\eqref{decoupleproblem},  the decoupled weight decay is a dynamic regularization along the training trajectory and could better regularize the loss. 
Compared with AdamW,  the advantages of Adan mainly come from its faster convergence  shown in Figure~\ref{fig:res-vit} (b).  We will discuss this below.

\begin{figure*}[t]
\centering
	\includegraphics[width=0.8\textwidth]{./pics/acc.pdf}
		\caption{Effects of momentum coefficients $(\beta_1,\beta_2,\beta_3)$ to top-1 accuracy (\%) of Adan on ViT-B under  MAE  training framework (800 pretraining and  100  fine-tuning epochs on ImageNet). 
}\label{fig:MAE}
\end{figure*}

\begin{table}[t]
 	\caption{ Top-1 ACC. (\%) of different optimizers for ViT-S  on ImageNet trained  under training setting II.  * is  from~\cite{touvron2021training}.\vspace{-0.5em}} \label{tab:vit-s}
 		%		\vspace{0.1em}
 		\label{tab:objectdetection}
 		\centering
 		\setlength{\tabcolsep}{10.0pt} % column spacing
 		
 		%\small{
 	{ \fontsize{8.3}{3}\selectfont{
\begin{tabular}{l|cccc}
	\toprule 
	Epoch              & 100  & 150     & 200     & 300     \\ \midrule
	AdamW~\cite{loshchilov2018decoupled} (default)   & 76.1 & 78.9    & 79.2    & 79.9$^*$    \\  
	Adam~\cite{kingma2014adam} & 62.0 & 64.0 &  64.5 & 66.7 \\
        Adai~\cite{xie2022adaptive} & 66.4 & 72.6 &  75.3 & 77.4 \\
	SGD-M~\cite{nesterov1983method,nesterov1988approach,nesterov2003introductory} & 64.3 & 68.7    & 71.4    & 73.9 \\ 
	
	LAMB~\cite{you2019large}            & 69.4 & 73.8    & 75.9    & 77.7 \\ 
	
	\textbf{Adan (ours)}               & \textbf{77.5} & \textbf{79.6}    & \textbf{80.0}    & \textbf{80.9}    \\
	\bottomrule
\end{tabular}
 	}}
\end{table}

\subsection{Ablation Study}\label{sec:robustness}

\begin{table*}[t!]
	\begin{minipage}[c]{.48\linewidth}
	\caption{Top-1 accuracy (\%) of ViT-S  on ImageNet trained under Training Setting I and II. $*$   is  reported in~\cite{touvron2021training}.} \label{tab:setting}
		\centering
		\setlength{\tabcolsep}{4.2pt} % column spacing
		
		{ \fontsize{8.3}{3}\selectfont{
\begin{tabular}{c|cc|cc}
	\toprule 
Training 	&   \multicolumn{2}{c}{Training Setting I}   &  \multicolumn{2}{c}{Training Setting II} \\
epochs	& AdamW~\cite{loshchilov2018decoupled} & {Adan} & AdamW~\cite{loshchilov2018decoupled} &  {Adan} \\ \midrule 
	150  & 76.4 &  \textbf{80.2} & 78.3 & \textbf{79.6} \\
	300  & 77.9 & \textbf{81.1} &~79.9$^*$ & \textbf{80.7}  \\
	\bottomrule
\end{tabular}
		}}
	\end{minipage}
	\hspace{1.3cm}
	\begin{minipage}[c]{.42\linewidth}
\caption{Top-1 accuracy (\%) of ViT-S and ConvNext-T  on ImageNet under  Training Setting II trained by 300 epochs.
} \label{tab:restart}
		\centering
		\setlength{\tabcolsep}{3.2pt} % column spacing
		%  row spacing
		{ \fontsize{8.3}{3}\selectfont{
\begin{tabular}{l|c|c}
	\toprule 
	& \multicolumn{1}{l|}{ViT Small {}} & \multicolumn{1}{l}{ConvNext Tiny } \\
	\midrule
	Adan w/o  restart   & 80.71                                             & 81.38                                      \\
	Adan w/ restart & \textbf{80.87}                                             & \textbf{81.62}   \\                          
	\bottomrule
\end{tabular}
		}}
	\end{minipage}%
\end{table*}

\subsubsection{Robustness to in momentum coefficients}
Here we choose MAE to investigate the effects of the momentum coefficients ($\beta$s) to Adan, since as shown in MAE, its pre-training is actually  sensitive to momentum coefficients of AdamW.  To this end,  following MAE, we  pretrain and fine tune ViT-B on ImageNet for 800 pretraining and 100  fine-tuning epochs.  We also fix one of $(\beta_1,\beta_2,\beta_3)$ and tune others.   
Figure \ref{fig:MAE} shows that by only pretraining 800 epochs, Adan  achieves $83.7\%+$ in most cases and outperforms the official accuracy $83.6\%$ obtained by AdamW with 1600 pretraining epochs, indicating the robustness of Adan to $\beta$s. We also  observe  1) Adan is not sensitive to  $\beta_2$;  2)  $\beta_1$ has a certain impact on Adan, namely the smaller the $(1.0-\beta_1)$, the worse the accuracy; 
3) similar to findings of MAE, a small second-order coefficient $(1.0-\beta_3)$ can improve the accuracy.  The smaller the $(1.0-\beta_3)$, the more current landscape information the optimizer would utilize to adjust the coordinate-wise learning rate.  Maybe the complex pre-training task of MAE is more preferred to the local geometric information. 

\subsubsection{Robustness to Training Settings}
Many works~\cite{liu2021swin,liu2022convnet,touvron2022deit,wightman2021resnet,touvron2021training} often preferably chose LAMB/Adam/SGD for Training Setting I and  AdamW for Training Setting II. Table \ref{tab:setting} investigates Adan under both settings and shows its consistent improvement.  Moreover, one can also observe that  Adan under Setting I largely improves the accuracy  of Adan under Setting II. It actually surpasses the best-known accuracy $80.4\%$ on ViT-small in \cite{touvron2022deit} trained by advanced layer scale strategy  and stronger data augmentation.

\subsubsection{Discussion on Restart Strategy}\label{restart}
Here we investigate the performance Adan with and without restart strategy on ViT and ConvNext under 300 training epochs.  From the results in Table~\ref{tab:restart}, one can observe that  restart strategy slightly improves the test performance of Adan. Thus, to make our Adan simple and avoid hyper-parameter tuning of the restart strategy (e.g., restart frequency), in all experiments except Table~\ref{tab:restart}, we do not use this restart strategy.

\section{Technical Proofs}
\subsection{Notation}\label{sec:notation}
We provide some notations that are frequently used throughout the paper.
The scale $c$ is in normal font. And the vector is in bold lowercase.
Give two vectors $\*x$ and $\*y$, $\*x\geq \*y$ means that $\qty(\*x-\*y)$ is a non-negative vector.
$\*x/\*y$ or $\frac{\*x}{\*y}$ represents the element-wise vector division.
$\*x \circ \*y$ means the element-wise multiplication, and
$\qty(\*x)^2 = \*x \circ \*x$.
$\innerprod{\cdot,\cdot}$ is the inner product.
Given a non-negative vector $\*n\geq 0$, we let $\norm{\*x}^2_{\sqrt{\*n}} \coloneqq \innerprod{\*x, \qty(\sqrt{\*n} + \varepsilon) \circ \*x}$.
Unless otherwise specified, $\norm{\*x}$ is the vector $\ell_2$ norm.
Note that $\E(\*x)$ is the expectation of random vector $\*x$.
For the functions $f(\cdot)$ and $g(\cdot)$, 
the notation $f(\epsilon)=\order{g(\epsilon)}$ means that $\exists a>0$, such that $ \frac{f(\epsilon)}{g(\epsilon)}\leq a, \forall \epsilon>0$.
The notation $f(\epsilon)=\Omega(g(\epsilon))$ means that $\exists a>0$, such that $\frac{f(\epsilon)}{g(\epsilon)}\geq a, \forall \epsilon>0$.
And $f(\epsilon)=\Theta(g(\epsilon))$ means that $\exists b\geq a>0$, such that $  a\leq \frac{f(\epsilon)}{g(\epsilon)}\leq b, \forall \epsilon>0$.

\subsection{Proof of Lemma \ref{lem:equivalence}: equivalence between the AGD and AGD II}\label{sec:AGDII}
In this section, we show how to get AGD II from AGD.
For convenience, we omit the noise term $\bm{\zeta}_k$.
Note that, let $\alpha \coloneqq 1-{\color{orange}\beta_1} $:
\[
\text{AGD:}
\left\{
\begin{aligned}
     & {\*g}_k = \nabla f(\bm{\theta}_{k} - \eta \alpha \*m_{k-1}) \\
     & \*m_k = \alpha \*m_{k-1} +  {\*g}_k \\
     &\bm{\theta}_{k+1} = \bm{\theta}_{k} - {\eta} \*m_k 
\end{aligned}
\right. .
\]
We can get:
\begin{equation}\label{eq:agd-reformulate}
    \begin{aligned}
     \bm{\theta}_{k+1} - \eta \alpha \*m_{k}  = &
     \bm{\theta}_{k} - {\eta} \*m_k - \eta \alpha \*m_{k}
      = \bm{\theta}_{k} - \eta \qty(1+\alpha)\qty(\alpha \*m_{k-1} +\nabla f(\bm{\theta}_{k} - \eta \alpha \*m_{k-1}))\\
      = & \bm{\theta}_{k} - \eta \alpha \*m_{k-1} - \eta \alpha^2 \*m_{k-1} - \eta\qty(1+\alpha)\qty(\nabla f(\bm{\theta}_{k} - \eta \alpha \*m_{k-1})).
\end{aligned}
\end{equation}
Let 
\[
\left\{
\begin{aligned}
& \Bar{\bm{\theta}}_{k+1} \coloneqq \bm{\theta}_{k+1} - \eta \alpha \*m_{k},\\
& \Bar{\*m}_{k} \coloneqq \alpha^2 \*m_{k-1} + (1+\alpha )\nabla f(\bm{\theta}_{k} - \eta \alpha \*m_{k-1}) = 
\alpha^2 \*m_{k-1} + (1+\alpha )\nabla f(\Bar{\bm{\theta}}_{k})\\
\end{aligned}
\right.
\]
Then, by Eq.\eqref{eq:agd-reformulate}, we have:
\begin{equation}\label{eq:AGDII-2}
  \Bar{\bm{\theta}}_{k+1} = \Bar{\bm{\theta}}_{k} - \eta \Bar{\*m}_{k}.  
\end{equation}
On the other hand, we have $\Bar{\*m}_{k-1} = 
\alpha^2 \*m_{k-2} + (1+\alpha )\nabla f(\Bar{\bm{\theta}}_{k-1})$ and :
\begin{equation}\label{eq:AGDII-1}
\begin{aligned}
\Bar{\*m}_{k} - \alpha \Bar{\*m}_{k-1}&  = 
\alpha^2 \*m_{k-1} + (1+\alpha )\nabla f(\Bar{\bm{\theta}}_{k})-\alpha \Bar{\*m}_{k-1}\\
& = (1+\alpha )\nabla f(\Bar{\bm{\theta}}_{k}) + \alpha^2 \qty(\alpha \*m_{k-2} + \nabla f(\Bar{\bm{\theta}}_{k-1}))-\alpha \Bar{\*m}_{k-1}\\
& = (1+\alpha )\nabla f(\Bar{\bm{\theta}}_{k}) + \alpha \qty(\alpha^2 \*m_{k-2} + \alpha \nabla f(\Bar{\bm{\theta}}_{k-1}) - \Bar{\*m}_{k-1}) \\
& = (1+\alpha )\nabla f(\Bar{\bm{\theta}}_{k}) + \alpha \qty(\alpha^2 \*m_{k-2} + \alpha \nabla f(\Bar{\bm{\theta}}_{k-1}))-\alpha \Bar{\*m}_{k-1}\\
& = (1+\alpha )\nabla f(\Bar{\bm{\theta}}_{k}) - \alpha \nabla f(\Bar{\bm{\theta}}_{k-1}) \\
& = \nabla f(\Bar{\bm{\theta}}_{k}) + \alpha\qty( \nabla f(\Bar{\bm{\theta}}_{k}) - \nabla f(\Bar{\bm{\theta}}_{k-1})). 
\end{aligned}
\end{equation}
Finally, due to Eq.\eqref{eq:AGDII-2} and Eq.\eqref{eq:AGDII-1}, we have:
\[
\left\{
\begin{aligned}
& \Bar{\*m}_{k} = \alpha \Bar{\*m}_{k-1} + \qty\Big(\nabla f(\Bar{\bm{\theta}}_{k}) + \alpha\qty( \nabla f(\Bar{\bm{\theta}}_{k}) - \nabla f(\Bar{\bm{\theta}}_{k-1})))\\
&\Bar{\bm{\theta}}_{k+1} = \Bar{\bm{\theta}}_{k} - \eta \Bar{\*m}_{k}
\end{aligned}
\right.
\]

\subsection{Convergence Analysis with Lipschitz Gradient}\label{sec:first-order}
Before starting the proof, we first provide several notations. 
Let ${F}_k(\bm{\theta})\coloneqq E_{\bm{\zeta}}[ f(\bm{\theta},\bm{\zeta})] + \frac{\lambda_k}{2}\norm{\bm{\theta}}_{\sqrt{\*n_k}}^2$ and $\mu\coloneqq {\sqrt{2}\beta_3 c_\infty}/{\varepsilon}$,
\[
\norm{\*x}^2_{\sqrt{\*n_k}} \coloneqq \innerprod{\*x, \qty(\sqrt{\*n_k}+\varepsilon)\circ \*x}, \quad \lambda_k =  \lambda\qty(1-\mu)^k, \quad
\Tilde{\bm{\theta}}_k \coloneqq \qty(\sqrt{\*n_k}+\varepsilon) \circ {\bm{\theta}}_k.
\] 
{
\begin{lemma}\label{lem:prox}
Assume $f(\cdot)$ is $L$-smooth.
For
\[
\bm{\theta}_{k+1} = \argmin_{\bm{\theta}} \qty(\frac{\lambda_k}{2}\norm{\bm{\theta}}_{\sqrt{\*n_k}}^2 + f(\bm{\theta}_k)+ \innerprod{\*u_k , \bm{\theta}-\bm{\theta}_k} + \frac{1}{2\eta}\norm{\qty(\bm{\theta}-\bm{\theta}_k)}_{\sqrt{\*n_k}}^2).
\]
With $\eta \leq \min\{ \frac{\varepsilon}{3L},\frac{1}{10\lambda}\}$, define $\*g_k \coloneqq  \nabla f(\bm{\theta}_{k})$, then we have:
\[
{F}_{k+1}(\bm{\theta}_{k+1}) \leq {F}_k(\bm{\theta}_{k}) - \frac{\eta }{4c_\infty}\norm{\*u_k + \lambda_k \Tilde{\bm{\theta}}_k}^2 +  \frac{\eta}{2{\varepsilon}}\norm{\*g_k - \*u_k}^2.
\]
\end{lemma}
\begin{proof}
We denote $\*p_k \coloneqq \*u_k/\qty(\sqrt{\*n_k}+\varepsilon)$. 
By the optimality condition of $\bm{\theta}_{k+1}$, we have
\begin{equation}\label{eq:eta-diff}
\lambda_k \bm{\theta}_{k} + \*p_k =
\frac{\lambda_k \Tilde{\bm{\theta}}_k + \*u_k}{\sqrt{\*n_k}+\varepsilon}
=  \frac{1+\eta \lambda_k}{{\eta}} \qty(\bm{\theta}_{k} - \bm{\theta}_{k+1}).
\end{equation}
%\zp{for the second equation in (1), there should be negative sign before the right side. That is, $\bm{\theta}_{k+1}-\bm{\theta}_{k} = -\frac{\bm{\eta}_k}{1+\lambda \bm{\eta}_k} \circ \qty(\*u_k + \lambda \bm{\theta}_k)$}
Then for $\eta \leq \frac{\varepsilon}{3L}$, we have:
\[
\begin{aligned}
& {F}_{k+1}(\bm{\theta}_{k+1}) \leq f(\bm{\theta}_{k} ) + \innerprod{\nabla f(\bm{\theta}_{k}), \bm{\theta}_{k+1}-\bm{\theta}_{k}} + \frac{L}{2}\norm{\bm{\theta}_{k+1}-\bm{\theta}_{k}}^2 + \frac{\lambda_{k+1}}{2}\norm{\bm{\theta}_{k+1}}_{\sqrt{\*n_{k+1}}}^2 \\
\overset{(a)}{\leq} & f(\bm{\theta}_{k} ) + \innerprod{\nabla f(\bm{\theta}_{k}), \bm{\theta}_{k+1}-\bm{\theta}_{k}} + \frac{L}{2}\norm{\bm{\theta}_{k+1}-\bm{\theta}_{k}}^2 +  \frac{\lambda_{k}}{2}\norm{\bm{\theta}_{k+1}}_{\sqrt{\*n_{k}}}^2\\
\overset{(b)}{\leq} & {F}_k(\bm{\theta}_{k}) + \innerprod{\bm{\theta}_{k+1}-\bm{\theta}_{k},\lambda_k\bm{\theta}_{k} + \frac{\*g_k}{\sqrt{\*n_k}+\varepsilon}}_{\sqrt{\*n_{k}}} + \frac{L/{\varepsilon}+\lambda_k}{2} \norm{\bm{\theta}_{k+1}-\bm{\theta}_{k}}_{\sqrt{\*n_{k}}}^2\\
 = & {F}_k(\bm{\theta}_{k}) + \frac{L/{\varepsilon}+\lambda_k}{2} \norm{\bm{\theta}_{k+1}-\bm{\theta}_{k}}_{\sqrt{\*n_{k}}}^2 +
 \innerprod{\bm{\theta}_{k+1}-\bm{\theta}_{k}, \lambda_k \bm{\theta}_{k} + \*p_k + \frac{\*g_k-\*u_k}{\sqrt{\*n_k}+\varepsilon}}_{\sqrt{\*n_{k}}}
\\
\overset{(c)}{=} & {F}_k(\bm{\theta}_{k}) + \qty(\frac{L/{\varepsilon}+\lambda_k}{2}-\frac{1+\eta \lambda_k}{{\eta}}) \norm{\bm{\theta}_{k+1}-\bm{\theta}_{k}}_{\sqrt{\*n_{k}}}^2 +
 \innerprod{\bm{\theta}_{k+1}-\bm{\theta}_{k},  \frac{\*g_k-\*u_k}{\sqrt{\*n_k}+\varepsilon}}_{\sqrt{\*n_{k}}}
\\
  \overset{(d)}{\leq} & {F}_k(\bm{\theta}_{k}) + \qty(\frac{L/{\varepsilon}}{2} - \frac{1}{\eta}) \norm{\bm{\theta}_{k+1}-\bm{\theta}_{k}}_{\sqrt{\*n_{k}}}^2 + \frac{1}{2\eta}\norm{\bm{\theta}_{k+1}-\bm{\theta}_{k}}_{\sqrt{\*n_{k}}}^2  + \frac{\eta}{2{\varepsilon}}  \norm{ \*g_k - \*u_k}^2\\ %+ 
\leq & {F}_k(\bm{\theta}_{k}) - \frac{1}{3\eta}\norm{\bm{\theta}_{k+1}-\bm{\theta}_{k}}_{\sqrt{\*n_{k}}}^2  + \frac{\eta}{2{\varepsilon}}  \norm{ \*g_k - \*u_k}^2 \\
\leq & {F}_k(\bm{\theta}_{k}) - \frac{\eta }{4c_\infty}\norm{\*u_k + \lambda_k \Tilde{\bm{\theta}}_k}^2 +  \frac{\eta}{2{\varepsilon}}\norm{\*g_k - \*u_k}^2 ,
\end{aligned}
\]
where (a) comes from the fact $\lambda_{k+1}(1-\mu)^{-1} = \lambda_{k}$ and Proposition \ref{prop:eta_diff}:
$
\qty(\frac{\sqrt{\*n_{k}} + \varepsilon }{\sqrt{\*n_{k+1}} + \varepsilon})_i \geq 1-\mu
$, which implies:
\[
\lambda_{k+1}\norm{\bm{\theta}_{k+1}}_{\sqrt{\*n_{k+1}}}^2 \leq \frac{\lambda_{k+1}}{1-\mu} \norm{\bm{\theta}_{k+1}}_{\sqrt{\*n_{k}}}^2 = \lambda_{k} \norm{\bm{\theta}_{k+1}}_{\sqrt{\*n_{k}}}^2,
\]
and (b) is from:
\[
\norm{\bm{\theta}_{k+1}}_{\sqrt{\*n_{k}}}^2 = \qty(\norm{\bm{\theta}_{k}}_{\sqrt{\*n_{k}}}^2 + 2 \innerprod{\bm{\theta}_{k+1}-\bm{\theta}_{k},\bm{\theta}_{k}}_{\sqrt{\*n_{k}}} + \norm{\bm{\theta}_{k+1}-\bm{\theta}_{k}}_{\sqrt{\*n_{k}}}^2),
\]
(c) is due to Eqn.~\eqref{eq:eta-diff}, and
for (d), we utilize:
\[
\innerprod{\bm{\theta}_{k+1}-\bm{\theta}_{k},  \frac{\*g_k-\*u_k}{\sqrt{\*n_k}+\varepsilon}}_{\sqrt{\*n_{k}}} \leq \frac{1}{2\eta}\norm{\bm{\theta}_{k+1}-\bm{\theta}_{k}}_{\sqrt{\*n_{k}}}^2 + \frac{\eta}{2{\varepsilon}}  \norm{ \*g_k - \*u_k}^2,
\]
the last inequality comes from the fact in Eqn.~\eqref{eq:eta-diff} and $\eta \leq \frac{1}{10\lambda}$, such that:
\[
\frac{1}{3\eta}\norm{\qty(\bm{\theta}_{k+1}-\bm{\theta}_{k})}_{\sqrt{\*n_{k}}}^2 = \frac{\eta}{3 \qty(\sqrt{\*n_{k}}+\varepsilon)\qty(1+\eta\lambda_k)}\norm{\*u_k + \lambda_k \Tilde{\bm{\theta}}_k}^2 \geq \frac{\eta}{4c_\infty}\norm{\*u_k + \lambda_k \Tilde{\bm{\theta}}_k}^2.
\]
\end{proof}
}
\begin{theorem}
Suppose Assumptions \ref{asm:Lsmooth} and \ref{asm:boundVar} hold. 
Let $c_l \coloneqq \frac{1}{c_\infty}$ and $c_u \coloneqq \frac{1}{{\varepsilon}}$.
With ${\beta_3 c_\infty}/{\varepsilon}\ll 1$,
\[
 \eta^2 \leq \frac{c_l\beta_1^2}{8c_u^3 L^2},  \quad \max\qty{\beta_1,\beta_2} \leq \frac{ c_l \epsilon^2}{96 c_u \sigma^2},\quad T \geq \max\qty{\frac{24 \Delta_0}{\eta c_l \epsilon^2},\frac{24 c_u \sigma^2}{\beta_1 c_l \epsilon^2}},
\]
where $\Delta_0 \coloneqq F(\bm{\theta}_{0}) - f^*$ and $f^* \coloneqq \min_{\bm{\theta}}\E_{\bm{\zeta}}[\nabla f(\bm{\theta}_k,\bm{\zeta})]$, then we let $\*u_k \coloneqq \*m_k + \qty(1-\beta_1)\*v_k$ and have:
\[
\frac{1}{T+1} \sum_{k=0}^T \^E\qty(\norm{\*u_k + \lambda_k \Tilde{\bm{\theta}}_k}^2) \leq \epsilon^2, 
\]
and 
\[
\frac{1}{T+1}\sum_{k=0}^T \^E \qty(\norm{\*m_k - \*g^{full}_k}^2) \leq \frac{\epsilon^2}{4}, \quad \frac{1}{T+1}\sum_{k=0}^T \^E \qty(\norm{\*v_k}^2) \leq \frac{\epsilon^2}{4}.
\]
Hence, we have:
\[
\frac{1}{T+1} \sum_{k=0}^T \^E\qty(\norm{\nabla_{\bm{\theta}_k} \qty(\frac{\lambda_k}{2}\norm{\bm{\theta}}_{\sqrt{\*n_k}}^2 + \E_{\bm{\zeta}}[\nabla f(\bm{\theta}_k,\bm{\zeta})])}^2) \leq 4\epsilon^2.
\]
\end{theorem}
\begin{proof}
For convince, we let $\*u_k \coloneqq \*m_k + \qty(1-\beta_1)\*v_k$ and ${\*g}^{full}_{k} \coloneqq \E_{\bm{\zeta}}[\nabla f(\bm{\theta}_k,\bm{\zeta})]$.
We have:
\[
\norm{\*u_k - \*g^{full}_k}^2 \leq 2 \norm{\*m_k - \*g^{full}_k}^2 + 2 \qty(1-\beta_1)^2 \norm{\*v_k}^2.
\]
By Lemma \ref{lem:prox}, Lemma~\ref{lem:mk}, and Lemma \ref{lem:vk},
we already have:
\begin{align}
&{F}_{k+1}(\bm{\theta}_{k+1}) \leq  {F}_{k}(\bm{\theta}_{k}) - \frac{\eta c_l}{4}\norm{\*u_k + \lambda_k \Tilde{\bm{\theta}}_k}^2 +{\eta c_u} \norm{\*g^{full}_k - \*m_k}^2 + {\eta c_u}\qty(1-\beta_1)^2 \norm{\*v_k}^2 , \label{eq:thm1:obj}\\
& \^E\qty(\norm{\*m_{k+1} - \*g^{full}_{k+1}}^2) \leq \qty(1-\beta_1)\^E\qty(\norm{\*m_{k} - \*g^{full}_{k}}^2) + \frac{\qty(1-\beta_1)^2L^2}{\beta_1} \^E\qty(\norm{\bm{\theta}_{k+1} - \bm{\theta}_{k}}^2) + {\beta_1^2 \sigma^2}\label{eq:thm1:mk}\\
& \^E\qty(\norm{\*v_{k+1}}^2) \leq \qty(1-\beta_2)\^E\qty(\norm{\*v_{k}}^2) + 2\beta_2 \^E\qty(\norm{{\*g}^{full}_{k+1} - {\*g}^{full}_{k}}^2)
+  {3\beta_2^2 \sigma^2} \label{eq:thm1:vk}
\end{align}
Then by adding Eq.\eqref{eq:thm1:obj} with $\frac{\eta c_u}{\beta_1} \times$ Eq.\eqref{eq:thm1:mk} and $\frac{\eta c_u \qty(1-\beta_1)^2}{\beta_2} \times$ Eq.\eqref{eq:thm1:vk}, we can get:
\[
\begin{aligned}
&\^E\qty(\Phi_{k+1}) \leq 
\^E\qty( \Phi_{k}  - \frac{\eta c_l}{4} \norm{\*u_k + \lambda_k \Tilde{\bm{\theta}}_k}^2 + \frac{\eta c_u}{\beta_1}\qty(\frac{\qty(1-\beta_1)^2L^2}{\beta_1} \norm{\bm{\theta}_{k+1} - \bm{\theta}_{k}}^2 + {\beta_1^2 \sigma^2}) )\\
 & + \frac{\eta c_u \qty(1-\beta_1)^2}{\beta_2} \^E\qty(2\beta_2 L^2 \norm{\bm{\theta}_{k+1} - \bm{\theta}_{k}}^2 + {3\beta_2^2 \sigma^2})\\
\leq & \^E\qty( \Phi_{k}  - \frac{\eta c_l}{4} \norm{\*u_k + \lambda_k \Tilde{\bm{\theta}}_k}^2 + \eta c_u L^2 \qty(\frac{\qty(1-\beta_1)^2}{\beta_1^2}+2\qty(1-\beta_1)^2) \norm{\bm{\theta}_{k+1} - \bm{\theta}_{k}}^2) + \qty(\beta_1 + 3\beta_2){\eta c_u \sigma^2}\\
\overset{(a)}{\leq} &  \^E\qty( \Phi_{k}  - \frac{\eta c_l}{4} \norm{\*u_k + \lambda_k \Tilde{\bm{\theta}}_k}^2 +  \frac{\eta c_u L^2}{\beta_1^2} \norm{\bm{\theta}_{k+1} - \bm{\theta}_{k}}^2) + { 4 \beta_m\eta c_u \sigma^2}\\
\overset{(b)}{\leq} &  \^E\qty( \Phi_{k} +\qty( \frac{(\eta c_u)^3L^2}{\beta_1^2}- \frac{\eta c_l}{4})  \norm{\*u_k + \lambda_k \Tilde{\bm{\theta}}_k}^2 ) + { 4 \beta_m\eta c_u \sigma^2}\\
\leq &  \^E\qty( \Phi_{k} - \frac{\eta c_l}{8}  \norm{\*u_k + \lambda_k \Tilde{\bm{\theta}}_k}^2 ) + { 4 \beta_m\eta c_u \sigma^2},
\end{aligned}
\]
where we let:
\[
\begin{aligned}
&\Phi_k \coloneqq {F}_k(\bm{\theta}_{k}) - f^* + \frac{\eta c_u}{\beta_1} \norm{\*m_{k} - \*g^{full}_{k}}^2 + \frac{\eta c_u\qty(1-\beta_1)^2}{\beta_2}\norm{\*v_k}^2,\\
& \beta_m = \max\qty{
\beta_1, \beta_2} \leq \frac{2}{3}, \quad 
\eta \leq \frac{c_l\beta_1^2}{8c_u^3 L^2},
\end{aligned}
\]
and for (a), when $\beta_1 \leq \frac{2}{3}$, we have:
\[
\frac{\qty(1-\beta_1)^2}{\beta_1^2}+2\qty(1-\beta_1)^2 < \frac{1}{\beta_1^2},
\]
and (b) is due to Eq.\eqref{eq:eta-diff} from Lemma \ref{lem:prox}.
And hence, we have:
\[
\sum_{k=0}^T\^E\qty(\Phi_{k+1}) \leq \sum_{k=0}^T\^E\qty(\Phi_k)  -\frac{\eta c_l}{8} \sum_{k=0}^T\norm{\*u_k + \lambda_k \Tilde{\bm{\theta}}_k}^2 + \qty(T+1){4\eta  c_u \beta_m \sigma^2}.
\]
Hence, we can get:
\[
\frac{1}{T+1} \sum_{k=0}^T \^E\qty(\norm{\*u_k + \lambda_k \Tilde{\bm{\theta}}_k}^2) \leq \frac{8 \Phi_0}{\eta c_l T} + \frac{32 c_u \beta \sigma^2}{c_l} = \frac{8 \Delta_0}{\eta c_l T} + \frac{8 c_u \sigma^2}{\beta_1 c_l T} + \frac{32 c_u \beta_m \sigma^2}{c_l} \leq \epsilon^2,
\]
where
\[
\Delta_0 \coloneqq F(\bm{\theta}_{0}) - f^*, \quad \beta_m \leq \frac{c_l \epsilon^2}{96 c_u \sigma^2},\quad T \geq \max\qty{\frac{24 \Delta_0}{\eta c_l \epsilon^2},\frac{24 c_u \sigma^2}{\beta_1 c_l \epsilon^2}}.
\]
We finish the first part of the theorem. From Eq.\eqref{eq:thm1:mk}, we can conclude that:
\[
\frac{1}{T+1}\sum_{k=0}^T \^E \qty(\norm{\*m_k - \*g^{full}_k}^2) \leq \frac{\sigma^2}{ \beta T} + \frac{L^2\eta^2 c_u^2  \epsilon^2}{\beta_1^2} + {\beta_1 \sigma^2} < \frac{\epsilon^2}{4}.
\]
From Eq.\eqref{eq:thm1:vk}, we can conclude that:
\[
\frac{1}{T+1}\sum_{k=0}^T \^E \qty(\norm{\*v_k}^2) \leq  2L^2\eta^2 c_u^2  \epsilon^2 + {3\beta_2 \sigma^2} < \frac{\epsilon^2}{4}.
\]
Finally we have:
\[
\begin{aligned}
& \frac{1}{T+1} \sum_{k=0}^T \^E\qty(\norm{\nabla_{\bm{\theta}_k} \qty(\frac{\lambda_k}{2}\norm{\bm{\theta}}_{\sqrt{\*n_k}}^2 + \E_{\bm{\zeta}}[ f(\bm{\theta}_k,\bm{\zeta})])}^2)\\
\leq & \frac{1}{T+1} \qty(\sum_{k=0}^T \^E\qty(2\norm{\*u_k + \lambda_k \Tilde{\bm{\theta}_k}}^2 + 4\norm{\*m_k - \*g^{full}_k}^2 + 4\norm{\*v_k}^2)) \leq 4\epsilon^2.
\end{aligned}
\]
Now, we have finished the proof.
\end{proof}

\subsection{Faster Convergence with  Lipschitz Hessian}\label{sec:second-order}
\input{name_ref}
\subsection{Auxiliary Lemmas}\label{sec:auxiliary}

\input{aux_lem}
